# Supplementary material for: "I Want to Figure Things Out": Supporting Exploration in Navigation for People with Visual Impairments
Source: arXiv:2211.16465 source file (2022-11-29)
Supplement: Supplementary file 1 [file v1.tex]

\section{ Perspective from Participants Favoring Guidance only}
\label{sec:theothers}
Our findings about VIPs who were satisfied with guidance based assistance, reinforce prior work that builds off of this perspective of those who prefer to be guided. 
%With respect to Active Engagement with the environment,  they 
Half of our participants (n=4) do not find a need for more exploration and thus are satisfied with the route-centered nature of guidance based assistance. 
Similarly, %for Getting Navigation Help from Non-VIP effectively, 
while they agree that non-VIPs are often unhelpful, they are unphased by external social pressures, and are eager to accept sighted guide assistance.
Finally, while they agree on the importance and utility of O\&M skills, they value convenience more and thus do not want to spend the effort to practice and develop these skills. 
Below, we discuss in further detail of the experiences of these participants. 

\subsection{Gathering Information From the Environment in a Self-Directed Manner.}
We found that the first means of exploration, gathering information in a self-directed manner, is not a priority for these participants.
For examaple, some of these participants (n=3) stated that learning about the layout is not as important as getting to the destination. 
They explained that they preferred to receive direct assistance from others -- either from sighted people or through a system. 
This reliance on sighted assistance meant that their decision to visit an unfamiliar environment was dependent on availability of sighted assistance, including their friends and family. \\\\
\begin{tabu} to \linewidth { X[l] X[27l] X[2l]}
 & \textit{``Usually for groceries, I ask somebody to assist me because [...] I feel like [the shape of the store is] really complicated to learn."} - \textbf{William} & \\
\end{tabu}
\vspace{0.2cm}\\\\
Interestingly, in some scenarios, a few of these participants (n=2) highlighted that even they sometimes ask for a general layout of the space. 
However, they shift quickly towards getting assistance as the space becomes more and more complex to navigate. 
We found a direct relationship between the speed of this shift towards assistance and the participant's confidence in their O\&M skills.  

Furthermore, they prefer to update their mental maps -- which consisted of routes, and not complete maps -- by asking for directions instead of exploring. 
For instance, Daniel described their approach: \\\\
\begin{tabu} to \linewidth { X[l] X[27l] X[2l]}
 & \textit{"Anything [that could be] as simple as finding a room that is not braille signed or a checkout counter [...] would require me to ask for directions."} - \textbf{Daniel} & \\
\end{tabu}
\vspace{0.2cm} \\\\

Finally, these participants (n=4) use landmark information to memorize specific  routes and not to create more complete mental maps of the environment as they explore independently. 
Consequently, existing approaches for route preview or route rehearsal serve this group of participants well. 
For instance, William highlighted this "route specific" behaviour: \\\\
\begin{tabu} to \linewidth { X[l] X[27l] X[2l]}
 & \textit{"I try to use the wall like a  landmark [or I use] the doors that are near. [I use them] to follow just a straight line. "} - \textbf{William} & \\
\end{tabu}
\vspace{0.2cm}\\\\
William further explained that he prefers the convenience of a sighted guide and thus prefers to receive assistance rather than explore and generate a mental map for himself.
This reinforces prior findings by \cite{dias2015indoor} on VIPs' use of non-visual cues and landmarks to inform their decisions during navigation.

\subsection{Getting Information from Others}
The second means of exploration, getting information from others, is also not a huge concern for these participants, as they are generally satisfied information provided by non-VIPs.
For example, our participants (n=4) prefer to receive a more closely guided form of assistance such as having the other person walk with them to the destination, or sighted guide assistance, requiring little to no information from non-VIPs.
Also, none of these participants mentioned discomfort due to social pressures, and were generally satisfied with receiving as much assistance as they are offered. 

However, they did report that non-VIPs often did not know how to assist them properly. 
For example, Lucas highlighted an unpleasant experience receiving bad help from a non-VIP:\\\\
\begin{tabu} to \linewidth { X[l] X[27l] X[2l]}
 & \textit{“I had somebody once when I was travelling grab the end of my cane and [try] to pull me along by my cane, and that’s not [the correct way to assist]”} - \textbf{Lucas} & \\
\end{tabu}
\vspace{0.2cm} \\\\
Thus, their experiences reinforced prior findings on the inadequacy of non-VIP assistance. 

\subsubsection{Maintain and Learn O\&M Skills.}
Finally, the third means of exploration, maintaining and learning O\&M skills, is generally not a main issue for these participants, albeit their experiences still support the skills' importance.
These participants (n=4) prefer sighted assistance over using their O\&M skills for navigation -- primarily due to convenience. 
However, all of them are aware of the importance of these skills.
In fact, a few (n=2) expressed their desire to obtain better O\&M training. 
For instance, Charles shared how he believed he would have benefited from further O\&M instruction:\\\\
\begin{tabu} to \linewidth { X[l] X[27l] X[2l]}
 & \textit{“I feel like I would have benefited [from O\&M training]. I don't want to feel like I'm overexaggerating, but [I would be] at least 10 times more [independent at navigating] if I just had that training. [I would have preferred the trainer] telling me, ‘Hey, here's where we're going. Here's what we're going to do. Here's how to do it properly.’ Instead of [having to rely on a sighted guide] just [telling me], ‘Hey, we're going here. Enjoy.’”} - \textbf{Charles} & \\
\end{tabu}
\vspace{0.2cm} \\\\
However, Charles was not eager to practice these skills independently, as he emphasized the necessity of receiving training from an instructor over being self taught. 
Nevertheless, our findings confirmed prior studies on the importance of O\&M skills for VIP navigation.
