# Supplementary material for: "I Want to Figure Things Out": Supporting Exploration in Navigation for People with Visual Impairments
Source: arXiv:2211.16465 source file (2022-11-29)
Supplement: Supplementary file 2 [file v2.tex]

\section{Formative study procedure}
\label{sec:formative-study}
We started with a formative study with two VIPs to gather an initial data sample of VIPs' experiences in exploring unfamiliar environments, with an aim to refine the interview protocol --- both the structure and the questions --- to effectively answer our two research questions.
We hosted the two VIPs, who are not trained in research, at our lab for several months and conducted multiple pilot interviews and brainstorming sessions, iteratively refining our interview protocol for the main study.
Through this process we gained two major insights, one relating to each research question.
With respect to RQ1, 
we learned that VIPs' information needs are sensitive to their navigation goal: exploration versus guidance. Since our goal is to identify VIPs' information needs for exploration, we restructured our interview protocol to deliberately ask VIPs to recall their prior visits to locations where they had no specific destination in mind, i.e., \textit{exploration}; and also to locations where they traversed to a specific destination within the environment, i.e., \textit{guidance}. 
With respect to RQ2, 
we learned that collaboration is a key aspect to VIPs' exploration strategies and that some of the challenges they face during exploration arise from these collaborations with other people. This insight led us to refine our interview questions to \textit{identify} these other people and to \textit{gauge their effect}, both positive and negative, on VIPs' ability to successfully explore unfamiliar environments. The formative study concluded with a refined interview protocol for our main study with VIPs, which we describe next.
